# Supplementary material for: EBIC: an evolutionary-based parallel biclustering algorithm for pattern discover
Source: arXiv:1801.03039 source file (2018-07-26)
Supplement: Supplementary file 1 [file supplementary-material.pdf]

# Supplementary Material

**EBIC: an evolutionary-based parallel biclustering algorithm for pattern discovery**

Patryk Orzechowski, Moshe Sipper, Xiuzhen Huang, Jason H. Moore

April 7, 2018

## Complexity Analysis of EBIC

The total time complexity of the sequential version of EBIC is on the order of $\mathcal{O}(bmnk)$, where m – number of columns, n – number of rows, k – number of iterations, and b – number of biclusters (size of the population). Taking into consideration the fact that EBIC exploits data parallelism, its complexity is reduced to $\mathcal{O}(bmnk/p)$, where p – number of processors.

The algorithm in each iteration sorts individuals based on their fitness, which takes up to $\mathcal{O}(kb \log b)$. Usually, $\log b << n$. The most time-consuming part of the algorithm is determining the fitness of the set of biclusters. This requires checking at every iteration, for each of the rows, the values of columns contained in CBF, which takes $\mathcal{O}(nmb)$.

The theoretical worst-case scenario of the algorithm is related to performing an exhaustive search on all combinations of columns. There are $2^m$ possible combinations. Thus, the worse-case time complexity of EBIC, when performing an exhaustive search on all combinations of columns, is on the order of $\mathcal{O}(mn2^m/p)$. Nonetheless, the actual complexity of the algorithm is much lower and driven by evolution, which allows to check only the most promising trends.

## Patterns of Biclusters

EBIC attempts to find order-preserving patterns in data. This means that after sorting a bicluster by columns, rows of the bicluster will have the same monotonous trend (i.e., for given rows, the values in the first columns are greater or equal than the values in the second column, which are greater or equal than the values in the third column, and so forth). EBIC also detects negative correlations. This means that those rows are also added to the bicluster, in which the relation is opposite (i.e., for rows, the values in the first column are lower or equal than the values in the second column, and so forth).

A sample pattern detected by EBIC in synthetic data can be found in the upper left corner of Fig. 1. For the majority of rows the pattern of the bicluster starts with low values (green color on left side of bicluster), then gradually increases to high values (red color on the right side of the bicluster). The negative correlations that are included in the bicluster can be found in top rows of the the bicluster and have high values (red color to the left), which gradually change to low values (green color to the right) with each consecutive column.

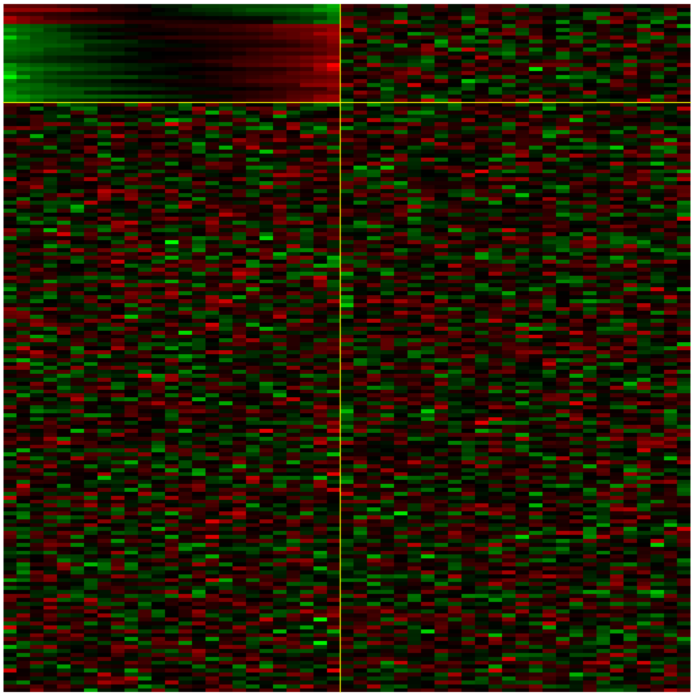

Figure 1: A heatmap with a sample bicluster detected by EBIC (see upper left corner). The rows and columns of the bicluster were rearranged in order to better demonstrate its pattern.

## Noise Resistance

In this section we discuss how noise influences the performance of our method. For each of the synthetic datasets, we generated three different datasets by adding random normally distributed noise $N(0, \sigma)$. We considered three levels, $\sigma = 0.1, 0.25, 0.5$. Thus, an additional 357 datasets were generated in total (119 datasets per each level of noise). We performed experiments using four different values of the tolerance parameter $\epsilon$: $\epsilon = 0.00001, 0.01, 0.05, 0.5$. All the previous tests in this study (on both synthetic and genomic datasets) were performed with tolerance parameter $\epsilon = 0.00001$.

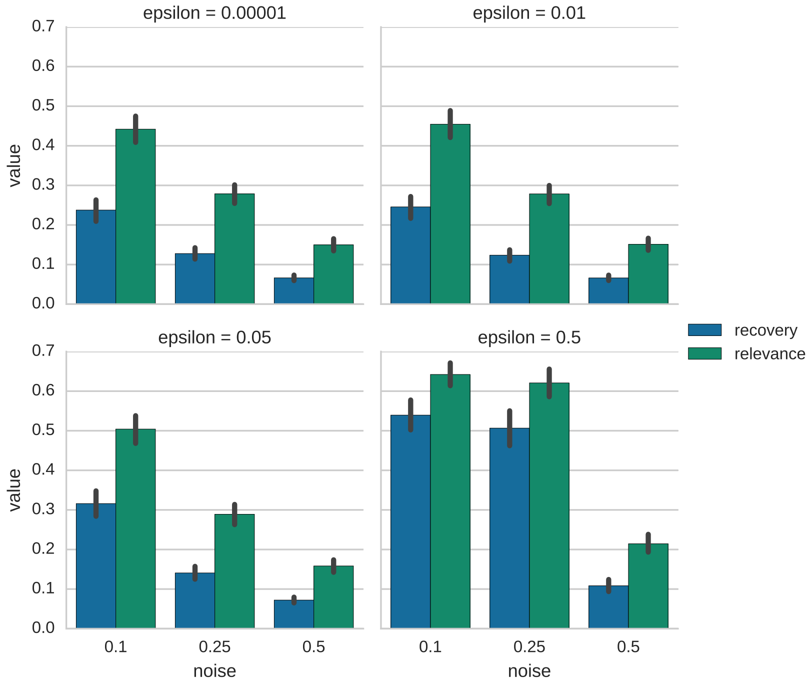


Figure 2: EBIC noise resistance. Each chart represents the recovery and relevance for three levels of noise added to the original dataset from a normal distribution $N(0, \sigma)$ with parameter $\sigma = 0.1, 0.25, 0.5$. Four values of a tolerance parameter $\epsilon$ are considered: 0.00001, 0.01, 0.05 and 0.5.

The results suggest that the tolerance parameter for synthetic datasets should be set to 0.5 in order to obtain better noise resistance for EBIC. Our method tolerates noise of up to $N(0, 0.25)$ and is still able to provide over 50% scores of recovery and relevance across all different problems. Assessment of the performance of the method with modified $\epsilon$ parameter requires further verification.

## Stopping Criterion for Genomic Datasets

We investigated the optimal stopping criterion for the algorithm on real genetic datasets. Using 8 GDS datasets we first allowed 20,000 iterations and noted how the percentage and number of enriched biclusters changed over time. The test was performed every 100 iterations. The results of our study are presented in Figs. 3 and 4 for the overlap threshold of 0.5 and Figs. 5 and 6 for the overlap threshold of 0.75, respectively. In each of the tests EBIC was allowed to return up to 400 biclusters in order to verify scores with better precision.

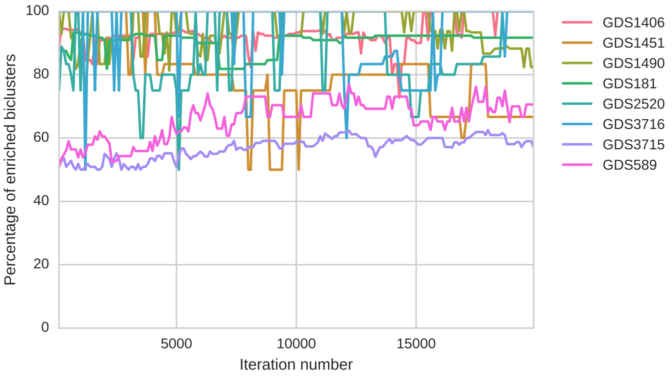


Figure 3: The change in the proportion of significantly enriched biclusters depending on the iteration number, with overlap ratio equal to 0.5.

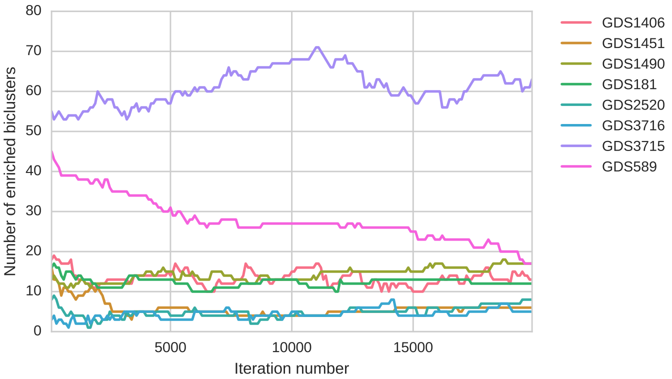


Figure 4: The change in the number of significantly enriched biclusters depending on the iteration number, with overlap ratio equal to 0.5.

The results are inconclusive. Some of the datasets already had a very high percentage of enriched biclusters starting at iteration 100. For example, all

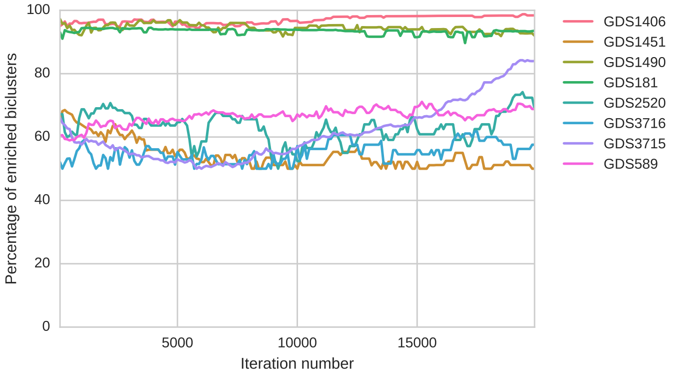


Figure 5: The change in the proportion of significantly enriched biclusters depending on the iteration number, with overlap ratio equal to 0.75.

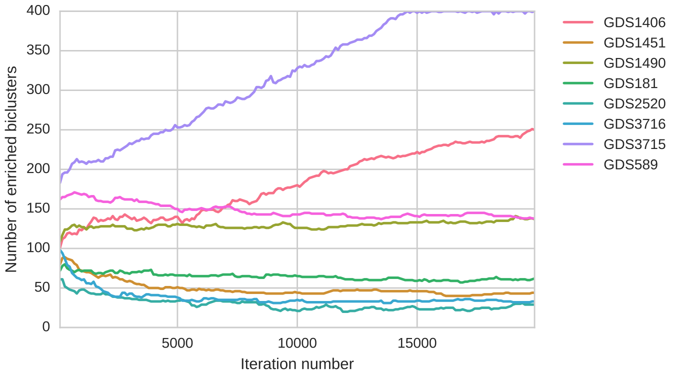


Figure 6: The change in the number of significantly enriched biclusters depending on the iteration number, with overlap ratio equal to 0.75.

biclusters were significantly enriched for GDS1451 and with new iterations the number dropped rather than increased. Dataset GDS1406, on the other hand, generally increased the percentage of significantly enriched biclusters over time.

## Penalty for Homogeneity of Columns

Maintaining high diversity in a population of a series of columns represented by CBF is crucial in order to be able to obtain substantially different biclusters. This is the major reason for applying a penalty for overusing the same column within the population. The penalty allows to reproduce the same column across multiple individuals while reducing the chances of accepting a new individual that is not sufficiently different from the previously allowed individuals.

In order to determine the penalty that should be applied to each individual attempted to be added to the population, we applied 4 different values of the threshold that is used to penalize for homogeneity in the population of CBF columns. We first tested 5000 iterations, starting from the same seed. A homogeneity threshold equal to 1.0 represented the scenario in which no penalty is applied for reusing the same columns in the population. The average recovery and relevance scores are presented in Fig. 7.

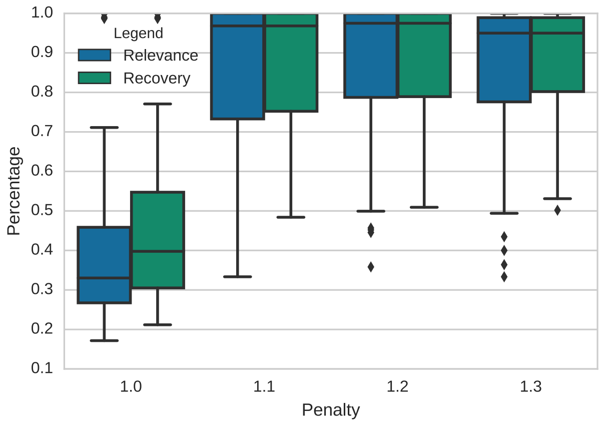


Figure 7: Average relevance and recovery for discovering 6 major biclustering patterns. Four different values of the homogeneity threshold are tested, with threshold equal to 1.0 meaning no penalty applied.

The highest average relevance and recovery was obtained using a homogeneity threshold of 1.2 and this value was used as a default in our method.
